# Supplementary material for: When Prompt-based Incremental Learning Does Not Meet Strong Pretraining
Source: arXiv:2308.10445 ancillary file (2023-08-21)
Supplement: Supplementary file 1 [file supplement.pdf]

# Supplementary material for “When Prompt-based Incremental Learning Does Not Meet Strong Pretraining”

Yu-Ming Tang<sup>1,3</sup>

Yi-Xing Peng<sup>1,3</sup>

Wei-Shi Zheng<sup>1,2,3\*</sup>

<sup>1</sup>School of Computer Science and Engineering, Sun Yat-sen University, China

<sup>2</sup>Peng Cheng Laboratory, Shenzhen, China

<sup>3</sup>Key Laboratory of Machine Intelligence and Advanced Computing, Ministry of Education, China

{tangym9, pengyx23}@mail2.sysu.edu.cn

wszheng@ieee.org

## Abstract

*This supplementary material is for our main manuscript “When Prompt-based Incremental Learning Does Not Meet Strong Pretraining”. To provide more details of our main paper, this material contains the following contents. Firstly, we conduct experiments on satellite data which has a semantic gap from the ImageNet dataset to show the necessity of our method (Sec. A1). Secondly, we show the detailed structure of the proposed Adaptive Prompt Generator (APG) in Sec. A2. Then, we detail the backbone adjustment in Sec. A3 and analysis of computation costs and extra parameters of the APG are shown in Sec. A4. We also provide comparisons with other prompted-based methods on ImageNet-R with Tiny-ImageNet pretrained weights in Sec. A5 corresponding to Sec. 4.3 in the main manuscript. Furthermore, corresponding to Sec. 4.4 in the main manuscript, we also provide ablation studies and analysis on CIFAR100 in Sec. A6 and Sec. A7. For a more intuitive illustration of the generated prompts, we conduct t-SNE [9] illustration of the generated prompts during different tasks of incremental learning in Sec. A8.*

## A1. The necessity of the proposed method

As stated in the main text, we proposed a more general prompted-based incremental learning method that does not rely on intensively pretrained backbones. Our work is not to refuse using any pretrained backbones, but to make it possible to learn incrementally when facing sequential tasks that are largely different from the pretrained task. To further show the necessity of our method, we conduct experiments on the EuroSAT [4] and NWPU-RESISC45 [1] datasets (satellite data), which are largely different from the pretrain-

ing domain (ImageNet-21k). For both two datasets, we split the original dataset with the ratio of 80(training set)-20(test set). For EuroSAT, we construct 5 incremental tasks under the basic class-increment protocol in which each task contains 2 classes for learning. Similarly, we construct 9 tasks for NWPU-RESISC45, where each task contains 5 classes.

| Dataset  | #Classes | #Samples |
|----------|----------|----------|
| EuroSAT  | 10       | 27,000   |
| RESISC45 | 45       | 31,500   |

Table A1. Details of two satellite datasets.

The results in Table A2 show that (a) previous methods perform poorly and fall far behind the performance upper bound which is fine-tuning the model on the whole dataset; (b) our method significantly outperforms previous methods. This indicates that prior prompt-based works are not suitable for incremental tasks that are largely different from the pretrained task (*i.e.* the semantic gap mentioned in the main paper.) and our method can effectively reduce the negative effects of this gap.

| methods    | Pretrained Type | RESISC45 (B0-T9) |              | EuroSAT (B0-T5) |              |
|------------|-----------------|------------------|--------------|-----------------|--------------|
|            |                 | Avg Acc.         | Last         | Avg. Acc.       | Last         |
| Finetune   | I-21k           | -                | 96.60        | -               | 97.46        |
| L2P        | I-21k           | 69.74            | 56.67        | 73.22           | 54.62        |
| DualPrompt | I-21k           | 74.66            | 66.30        | 82.38           | 71.22        |
| Ours       | I-21k           | <b>88.73</b>     | <b>88.00</b> | <b>85.94</b>    | <b>84.60</b> |

Table A2. Experiments on two domains that have a huge gap from the ImageNet. Finetune means fine-tuning the pretrained model on the whole dataset. I-21k means models are pretrained on ImageNet-21k. Average accuracy (Avg Acc.) and accuracy on the last task (Last) are reported.

\*Corresponding author

## A2. Details of the Proposed Adaptive Prompt Generator (APG)

In the main paper, the proposed Adaptive Prompt Generator (APG) is used to adaptively generate prompts for the main network. The APG consists of three components: two projection modules for input/output and the cross-attention module. An illustration of the APG is shown in Fig. A1. Taking the input feature (the intermediate feature of the main network), the projection module is used to project the feature into a shared space. The projection module consists of two fully-connected layers (FC). To preserve the information in the feature, we keep the dimension  $d$  of the input feature. For example, for the comparison with the models trained from scratch (Sec.4.2 in the main paper), we use  $d = 256$  and the weights in both FCs are  $W_{FC} \in \mathbb{R}^{256 \times 256}$ . The key component in the APG is the cross-attention module. We maintain a prompt candidate list for knowledge accumulation. The candidate list consists of a list of tokens  $\mathbf{I}_{Pcan} = [\hat{\mathbf{P}}_1, \dots, \hat{\mathbf{P}}_i, \dots, \hat{\mathbf{P}}_c]$ , where  $\hat{\mathbf{P}}_i \in \mathbb{R}^d$  shares the same dimension of the input feature and  $c$  is the number of classes learned. A multi-head cross-attention is shown in the lower left corner in Fig. A1. We use multi-head cross-attention to generate each prompt as stated in the main paper. The cross-attention operation is used to gather knowledge from different tasks. Instead of using the raw output of the cross-attention as the final output of the APG, we further apply a projection module. The output projection module is with the same structure as the input one.

## A3. Details of the Adjusted Backbone

We use the vanilla Vision Transformer (ViT) as our backbone due to its simplicity and versatility. To fairly compare with standard class-incremental learning models without pretraining, such as PODNet [3], DER [13], CwD [6], Foster [10], AFC [5], Imagine [7], which use the ResNet-18 as the backbone, we slightly modified the configuration of ViT. Specifically, we adjust the number of heads and the embedding dimension to match the parameter of the ResNet-18. A detailed configuration of our backbone is shown in Table A3. Note that, in Sec. 4.3 of the main paper, we compare our method with L2P and DualPrompt with the pre-trained backbone. In those experiments, we follow L2P [12] and dualprompt [11] using ViT-Base as our backbone.

## A4. Analysis of computation costs and extra parameters of the proposed APG

The proposed APG is a lightweight generator. For ResNet18-scale ViT (the default backbone in the main paper, see Section A3 for more details), the corresponding APG takes about 0.0137 GFLOPs which is negligible as the whole backbone takes 2.14 GFLOPs. For ViT-base which

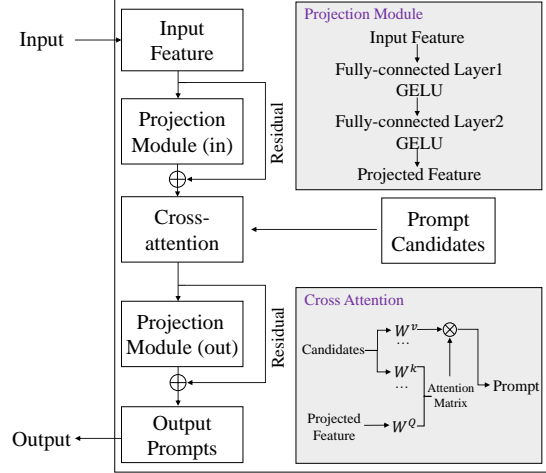

Figure A1. Detailed implementation of the proposed APG. The APG consists of three parts: the input projection, cross-attention operation and the output projection. The details of projection modules are shown in the upper left and the lower left shows a multi-head cross-attention operation for generating each prompt. Associated with the cross-attention operation, we maintain a prompt candidate list for knowledge aggregation.  $\otimes$  denotes the matrix multiplication,  $\oplus$  indicates the residual connection, and ‘GELU’ is the activation function.

| Model           | Embed Dim | #Heads | #Layers | #Params | Train Resolution |
|-----------------|-----------|--------|---------|---------|------------------|
| Vit-Tiny [8]    | 192       | 3      | 12      | 5M      | 224              |
| Vit-Small [8]   | 384       | 6      | 12      | 22M     | 224              |
| Vit-Base [2, 8] | 768       | 12     | 12      | 86M     | 224              |
| ResNet-18       | 512       | -      | -       | 11M     | 224              |
| Ours            | 256       | 8      | 12      | 10M     | 224              |

Table A3. Details of the adjusted backbone. We slightly adjust the vanilla ViT for matching the parameters of the ResNet-18.

takes 17.58 GFLOPs, our APG takes only 0.24 GFLOPs.

By default, the proportion of the number of parameters in APG to the backbone remains about 3% regardless of different scales of backbones since the feature dimension of APG is related to that of the backbone.

When expanding the candidate list during incremental learning, the extra memory cost is negligible. For each class, only one d-dim token is added to the prompt list. For example, in ViT-base ( $d=768$ , #Param=87M), expanding the prompt candidate list for 1000 classes costs only 0.768M parameters.

## A5. Incremental Learning on ImageNet-R with Pretrained Weights

Corresponding to Sec. 4.3 in the main paper, we make comparisons with L2P [12] and DualPrompt [11] with Tiny-ImageNet pretrained weights. Specifically, when with Tiny-ImageNet pretrained weights, our method achieves 5% and 5% higher accuracy compared with DualPrompt and L2P.

| Methods                          | ImageNet-R<br>B0-T5 |                | ImageNet-R<br>B0-T10 |                | ImageNet-R<br>B0-T20 |                |
|----------------------------------|---------------------|----------------|----------------------|----------------|----------------------|----------------|
|                                  | A $\uparrow$        | F $\downarrow$ | A $\uparrow$         | F $\downarrow$ | A $\uparrow$         | F $\downarrow$ |
| <i>ImageNet-21K Pretraining</i>  |                     |                |                      |                |                      |                |
| Upper Bound                      | 77.47               | -              | 77.87                | -              | 78.90                | -              |
| FT                               | 37.73               | 46.23          | 24.76                | 63.14          | 18.66                | 72.35          |
| L2P [12]                         | 66.86               | 5.02           | 66.61                | 9.37           | 64.08                | 8.64           |
| DualPrompt [11]                  | <b>73.02</b>        | 3.73           | 72.57                | 4.68           | 70.48                | 7.47           |
| Ours                             | 72.36               | 6.37           | <b>73.27</b>         | 8.59           | <b>71.22</b>         | 7.39           |
| <i>Tiny-ImageNet Pretraining</i> |                     |                |                      |                |                      |                |
| Upper Bound                      | 77.48               | -              | 78.35                | -              | 78.85                | -              |
| FT                               | 37.74               | 46.23          | 24.76                | 63.61          | 16.08                | 72.34          |
| L2P [12]                         | 73.26               | 5.66           | 71.94                | 6.32           | 70.84                | 8.74           |
| DualPrompt [11]                  | 72.78               | 3.22           | 72.15                | 3.39           | 69.81                | 3.91           |
| Ours                             | <b>73.78</b>        | 4.74           | <b>75.57</b>         | 6.78           | <b>74.45</b>         | 8.54           |

Table A4. Comparison to state-of-the-art prompt-based methods with ImageNet-21k/Tiny-ImageNet pretrained weights on ImageNet-R. The best and the second best results are marked in **bold**. ‘A’ means Avg. Acc and ‘F’ indicates the forgetting metric.

| Configs | w/o APG             |                      | w/ APG               |                      |                     | Avg. Acc.(%) |
|---------|---------------------|----------------------|----------------------|----------------------|---------------------|--------------|
|         | $\mathcal{L}_{cls}$ | $\mathcal{L}_{conC}$ | $\mathcal{L}_{conA}$ | $\mathcal{L}_{attn}$ | $\mathcal{L}_{tri}$ |              |
| c-1     | ✓                   |                      |                      |                      |                     | 17.09        |
| c-2     | ✓                   | ✓                    |                      |                      |                     | 46.12        |
| c-3     | ✓                   | ✓                    | ✓                    |                      |                     | 67.21        |
| c-4     | ✓                   | ✓                    | ✓                    | ✓                    |                     | 67.49        |
| c-5     | ✓                   | ✓                    | ✓                    |                      | ✓                   | 67.46        |
| c-6     | ✓                   | ✓                    |                      | ✓                    | ✓                   | 64.98        |
| Full    | ✓                   | ✓                    | ✓                    | ✓                    | ✓                   | <b>67.53</b> |

Table A5. Effectiveness of each loss function of the proposed method. ‘c-x’ denotes different training configs. ‘Full’ indicates the default full model. Experiments are conducted on CIFAR100 under the 10-tasks setting. The best result is marked in **bold**.

## A6. Ablation Studies on CIFAR100

In this section, we will discuss the ablation studies on CIFAR100. To illustrate the effectiveness of each component proposed in the APG, we ablate different losses and the results are shown in Table A5. Only with the classification loss  $\mathcal{L}_{cls}$ , the model face severe forgetting. This is mainly because the model is not able to maintain the learned knowledge without any samples kept as a memory. With the knowledge vector provided by the knowledge pool, the classifier is reminded by the loss  $\mathcal{L}_{conC}$ , and the forgetting is alleviated. With the proposed APG and the constraint loss  $\mathcal{L}_{conA}$ , the performance is boosted from 46.66% to 67.21%. It demonstrates that, with the knowledge pool, our proposed APG can adaptively aggregate knowledge from the old and new tasks and therefore can tackle knowledge degradation. With the attention constraint  $\mathcal{L}_{attn}$ , the performance increases to 67.49% and this shows that the constraint helps the APG to aggregate old knowledge. Furthermore, with the triplet loss  $\mathcal{L}_{tri}$  used to help the APG to generate class-specific prompts, the performance is boosted to 67.53%.

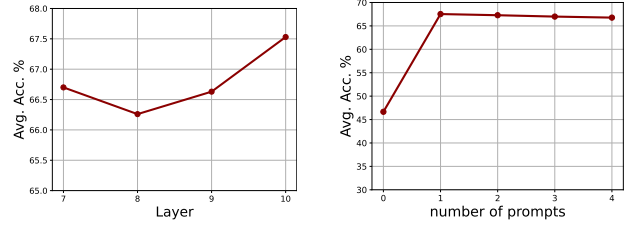

(a) The impact of which layers that APG augments into. (b) The impact of the number of generated prompts.

Figure A2. We conduct experiments on the impact of the layer of equipping the APG (a) and the impact of the number of prompts generated (b). All experiments are conducted on CIFAR100 at 10-task incremental learning setting.

## A7. Further Analysis on CIFAR100

Corresponding with Sec.4.5 in the main paper, we also conduct analyses of our model on CIFAR100. To investigate the impact of the position where the APG is equipped, we conduct several experiments on CIFAR100 under different  $l \in \{7, 8, 9, 10\}$ . We observe from Fig. 2(a) that when  $l = 10$  the performance is better than  $l = 7, 8, 9$ . This is mainly because the shallow layers output an intermediate feature that is not discriminative enough for generating class-specific prompts. We choose  $l = 10$  as our default setting. Similar to experiments on ImageNet-Subset in the main paper, we also conduct experiments about the impact of the number of generated prompts on CIFAR100. The results are shown in Fig. 2(b). When the number of prompts  $n > 0$ , the performance is boosted to around 67%, and when  $n$  increases, the performance drops slightly. We argue that it is mainly because the prompt generation is powerful and only 1 prompt is enough for instructing deeper layers considering that our backbone only has 10M parameters.

## A8. Visualization

In this section, we use t-SNE [9] to visualize our generated prompts to illustrate that our APG can generate class-specific prompts to instruct deeper layers. To illustrate the learning process of incremental learning, we visualize prompts generated in tasks 7 to 10 of the 10-tasks incremental learning on ImageNet-Subset. The visualization results are in Fig. A3. We use the testing set of the ImageNet-subset to generate prompts. It can be observed from the figure that most of the generated prompts are class-specific and the prompts are clustered based on the class of the input feature. Furthermore, the old knowledge is preserved well during the incremental learning process, and the prompts of old tasks are still class-specific across tasks, e.g. class 5, 25, 40, 51, etc. Moreover, prompts of the newly introduced classes are well-separated from the old ones. We can observe from the figure that newly-introduced classes 86,

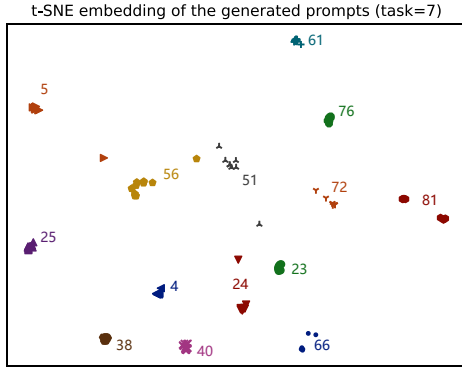

(a) t-SNE visualization of the generated prompts at  $\mathcal{T}_7$ .

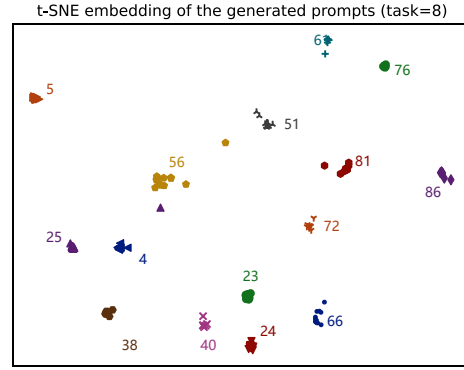

(b) t-SNE visualization of the generated prompts at  $\mathcal{T}_8$ .

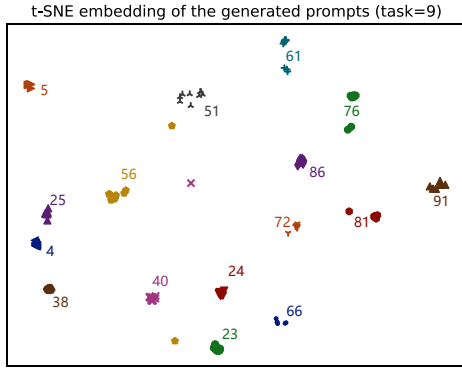

(c) t-SNE visualization of the generated prompts at  $\mathcal{T}_9$ .

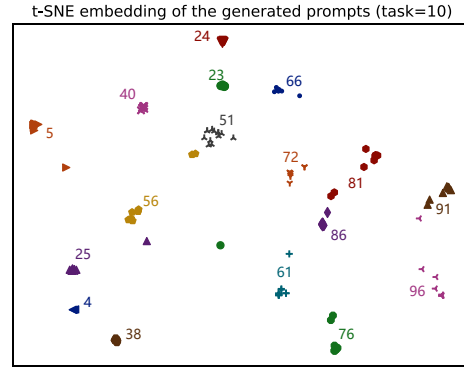

(d) t-SNE visualization of the generated prompts at  $\mathcal{T}_{10}$ .

Figure A3. t-SNE visualization of generated prompts at tasks 7,8,9 and 10. We conduct experiments on ImageNet-subset in the 10-task incremental setting. The testing set of the ImageNet-subset is used to generate prompts. We randomly selected some classes and corresponding samples in the test set for visualization. We use different colors and different shapes to indicate different classes. Besides, we additionally annotate the class label to which each cluster belongs. Classes 86, 91 and 96 are newly-added classes in tasks 8,9 and 10. Best viewed in color and zoom in.

91 and 96 are separated from other old prompts and are also preserved well during the incremental learning. Last but not least, we also see that there are some prompts from two different classes that are close in the t-SNE space sometimes. We argue that this is mainly because such two classes have shared knowledge, so the prompts are close to each other. For example, class 51 and class 56 are jacamar (a kind of bird) and drake, which have similar attributes such as beak and feather. In conclusion, our APG successfully generates class-specific prompts and manages to maintain knowledge from old tasks.

## References

[1] Gong Cheng, Junwei Han, and Xiaoqiang Lu. Remote sensing image scene classification: Benchmark and state of the

art. *Proceedings of the IEEE*, 2017. 1

[2] Alexey Dosovitskiy, Lucas Beyer, Alexander Kolesnikov, Dirk Weissenborn, Xiaohua Zhai, Thomas Unterthiner, Mostafa Dehghani, Matthias Minderer, Georg Heigold, Sylvain Gelly, Jakob Uszkoreit, and Neil Houlsby. An image is worth 16x16 words: Transformers for image recognition at scale. In *International Conference on Learning Representations*, 2021. 2

[3] Arthur Douillard, Matthieu Cord, Charles Ollion, Thomas Robert, and Eduardo Valle. Podnet: Pooled outputs distillation for small-tasks incremental learning. In *Proceedings of the European Conference on Computer Vision*, 2020. 2

[4] Patrick Helber, Benjamin Bischke, Andreas Dengel, and Damian Borth. Eurosat: A novel dataset and deep learning benchmark for land use and land cover classification. *IEEE Journal of Selected Topics in Applied Earth Observations*

*and Remote Sensing*, 2019. 1

- [5] Minsoo Kang, Jaeyoo Park, and Bohyung Han. Class-incremental learning by knowledge distillation with adaptive feature consolidation. In *Proceedings of the IEEE/CVF Conference on Computer Vision and Pattern Recognition*, 2022. 2
- [6] Yujun Shi, Kuangqi Zhou, Jian Liang, Zihang Jiang, Jiashi Feng, Philip HS Torr, Song Bai, and Vincent YF Tan. Mimicking the oracle: An initial phase decorrelation approach for class incremental learning. In *Proceedings of the IEEE/CVF Conference on Computer Vision and Pattern Recognition*, 2022. 2
- [7] Yu-Ming Tang, Yi-Xing Peng, and Wei-Shi Zheng. Learning to imagine: Diversify memory for incremental learning using unlabeled data. In *Proceedings of the IEEE/CVF Conference on Computer Vision and Pattern Recognition*, 2022. 2
- [8] Hugo Touvron, Matthieu Cord, Matthijs Douze, Francisco Massa, Alexandre Sablayrolles, and Hervé Jégou. Training data-efficient image transformers & distillation through attention. In *International Conference on Machine Learning*, 2021. 2
- [9] Laurens Van der Maaten and Geoffrey Hinton. Visualizing data using t-sne. *Journal of machine learning research*, 2008. 1, 3
- [10] Fu-Yun Wang, Da-Wei Zhou, Han-Jia Ye, and De-Chuan Zhan. Foster: Feature boosting and compression for class-incremental learning. In *Proceedings of the European Conference on Computer Vision*, 2022. 2
- [11] Zifeng Wang, Zizhao Zhang, Sayna Ebrahimi, Ruoxi Sun, Han Zhang, Chen-Yu Lee, Xiaoqi Ren, Guolong Su, Vincent Perot, Jennifer Dy, et al. Dualprompt: Complementary prompting for rehearsal-free continual learning. In *Proceedings of the European Conference on Computer Vision*, 2022. 2, 3
- [12] Zifeng Wang, Zizhao Zhang, Chen-Yu Lee, Han Zhang, Ruoxi Sun, Xiaoqi Ren, Guolong Su, Vincent Perot, Jennifer Dy, and Tomas Pfister. Learning to prompt for continual learning. In *Proceedings of the IEEE/CVF Conference on Computer Vision and Pattern Recognition*, 2022. 2, 3
- [13] Shipeng Yan, Jiangwei Xie, and Xuming He. Der: Dynamically expandable representation for class incremental learning. In *Proceedings of the IEEE/CVF Conference on Computer Vision and Pattern Recognition*, 2021. 2
